# Supplementary material for: Provably Robust Adversarial Examples
Source: arXiv:2007.12133 source file (2022-03-17)
Supplement: Supplementary file 1 [file overview_figure.tex]

\begin{figure*}[t]
\vskip -3em
\centering

\def \minw {40mm}
\def \minh {55mm}
\makeatletter
\newcommand{\stepbox}[6]{
	\ifblank{#1} {\node}{node} (#2)
	[draw=black!60, fill=black!05, rectangle, rounded corners=2pt,
	minimum width=\minw, minimum height=\minh,anchor=north west, #3] at (#4, #5) {#6}
}
\makeatother
\makeatletter
\newcommand{\gettikzx}[2]{%
	\tikz@scan@one@point\pgfutil@firstofone#1\relax
	\edef#2{\the\pgf@x}%
}
\makeatother
\makeatletter
\newcommand{\gettikzy}[2]{%
	\tikz@scan@one@point\pgfutil@firstofone#1\relax
	\edef#2{\the\pgf@y}%
}
\makeatother

\makeatletter      
\newcommand{\getAngle}[3]{%
	\pgfmathanglebetweenpoints{\pgfpointanchor{#1}{center}}
	{\pgfpointanchor{#2}{center}}
	\pgfmathsetmacro{#3}{\pgfmathresult}
}
\makeatother

\makeatletter      
\newcommand{\getDistance}[4]{%
	\getAngle{#2}{#1}{\anglep}
	\getAngle{#2}{#3}{\anglel}
	\gettikzx{(#1)}{\vx}
	\gettikzy{(#1)}{\vy}
	\gettikzx{(#2)}{\lx}
	\gettikzy{(#2)}{\ly}
	\pgfmathveclen{\vx-\lx}{\vy-\ly}
	\pgfmathsetmacro{\lenp}{\pgfmathresult}
	\pgfmathparse{sin(\anglep - \anglel)*\lenp}
	\edef#4{\pgfmathresult pt}
}
\makeatother

\makeatletter      
\newcommand{\myoffsetBy}[6]{%
	\gettikzx{(#1)}{\vxo}
	\gettikzy{(#1)}{\vyo}
	\gettikzx{(#2)}{\lx}
	\gettikzy{(#2)}{\ly}
	\pgfmathveclen{\vxo-\lx}{\vyo-\ly}
	\pgfmathsetmacro{\leno}{\pgfmathresult}
	
	\gettikzx{(#3)}{\vxt}
	\gettikzy{(#3)}{\vyt}
	\pgfmathveclen{\vxt-\lx}{\vyt-\ly}
	\pgfmathsetmacro{\lent}{\pgfmathresult}
	
	\pgfmathparse{#4}
	\edef#5{\pgfmathresult pt}
	\pgfmathsetmacro{\offseto}{\pgfmathresult}
	\pgfmathparse{#4/\leno*\lent}
	\edef#6{\pgfmathresult pt}
	\pgfmathsetmacro{\offsett}{\pgfmathresult}
}
\makeatother

\newcommand{\subfigtitle}[3]{
	\begin{tiny}
		\begin{tabular}{l@{\hspace{1em}}l@{}}
			#1. & #2\\
			& #3
		\end{tabular}
	\end{tiny}
}

\scalebox{0.8}{\begin{tikzpicture}[font=\small\sffamily]
	\tikzset{>=latex}
	
	\stepbox{}{step3}{minimum width=\minw*3+10mm, anchor=north west}{\minw + 3.5mm}{0}{GetPoly};
	
	\node[anchor=west] (gen1) at ($(step3.west) + (2mm, 0)$) {\input{overview_figure/genpoly1.tex}};
	\node[anchor=east] (gen3) at ($(step3.east) + (-2mm, 0)$) {\input{overview_figure/genpoly3.tex}};
	\node[anchor=center] (gen2) at ($0.5*(gen3.east) + 0.5*(gen1.west)$) {\input{overview_figure/genpoly2.tex}};
	
	\node[anchor=east] (under3) at ($(step3.west) + (-3mm, 0)$) {\input{overview_figure/underapprox3.tex}};
	
	\node[anchor=north] (poly0) at ($(step3.north) + (0, -2mm)$) {\begin{normalsize}Polyhedral Region\end{normalsize}};
	
	\node[anchor=north] (poly0) at ($(gen1.south) + (0, 1mm)$) {\subfigtitle{1}{Try to verify the network}{and obtain hyperplanes}};
	\node[anchor=north] (poly0) at ($(gen2.south) + (0, 1mm)$) {\subfigtitle{2}{Adjust hyperplanes' biases until they do}{not intersect the underapproximation box}};
	\node[anchor=north] (poly0) at ($(gen3.south) + (0, 1mm)$) {\subfigtitle{3}{Repeat until the polyhedral}{region is verifiable}};

	\path[->]  ($(under3.east) + (1mm,0)$) edge node [below] {\begin{scriptsize}Initialize\end{scriptsize}} ($(gen1.west) + (4mm,0)$);  
	
	\path[->] ($(gen2.west)+(4mm,-2mm)$) edge[bend left] node [below] {\begin{scriptsize}Get Planes\end{scriptsize}} ($(gen1.east)+(0mm,-1.5mm)$);
	\path[->]  ($(gen1.east)+(0,2mm)$) edge[bend left] node [above] {\begin{scriptsize}Adjust Planes\end{scriptsize}} ($(gen2.west)+(4mm,1.5mm)$);
	
	\path[->] ($(gen2.east) + (1mm,0)$) edge node [below] {\begin{scriptsize}Verifies\end{scriptsize}} ($(gen3.west) + (4mm,0)$);

\end{tikzpicture}}
\caption{Overview of our method for generating provably robust polyhedral adversarial examples. The green triangle denoted $\mathcal{T}$ represents the ground truth adversarial region. The dashed blue rectangle denoted $\mathcal{O}$ and the violet dotted rectangle denoted $\mathcal{U}$ represent the fitted overapproximation and underapproximation boxes, respectively. The solid black lines represent hyperplanes generated by the certification procedure \verifier{}, while their dash-dotted counterparts represent the hyperplanes after bias-adjustment. The small arrows going out of the hyperplanes in Step 1 and Step 2 represent the direction which is retained by the hyperplanes' corresponding half-spaces. The output polyhedral region denoted $\mathcal{P}$ is shown in red in Step 3.}
\vskip -0.1in
\label{fig:overview_appendix}
\end{figure*}
